# Supplementary material for: Limitations of ab initio methods to predict the electronic-transport properties of two-dimensional materials: The computational example of 2H-phase transition metal dichalcogenides
Source: arXiv:1912.03795 source file (2019-12-09)
Supplement: Supplementary file 1 [file supplimental.pdf]

**Supplemental material: Limitations of *ab initio* methods to  
predict the electronic-transport properties of two-dimensional  
materials: The computational example of 2H-phase transition  
metal dichalcogenides**

Gautam Gaddemane,<sup>1</sup> Sanjay Gopalan,<sup>1</sup> Maarten L. Van de Put,<sup>1</sup> and Massimo V. Fischetti<sup>1</sup>

<sup>1</sup>*Department of Materials Science and Engineering, The University of Texas at Dallas  
800 W. Campbell Rd., Richardson, TX 75080, USA*

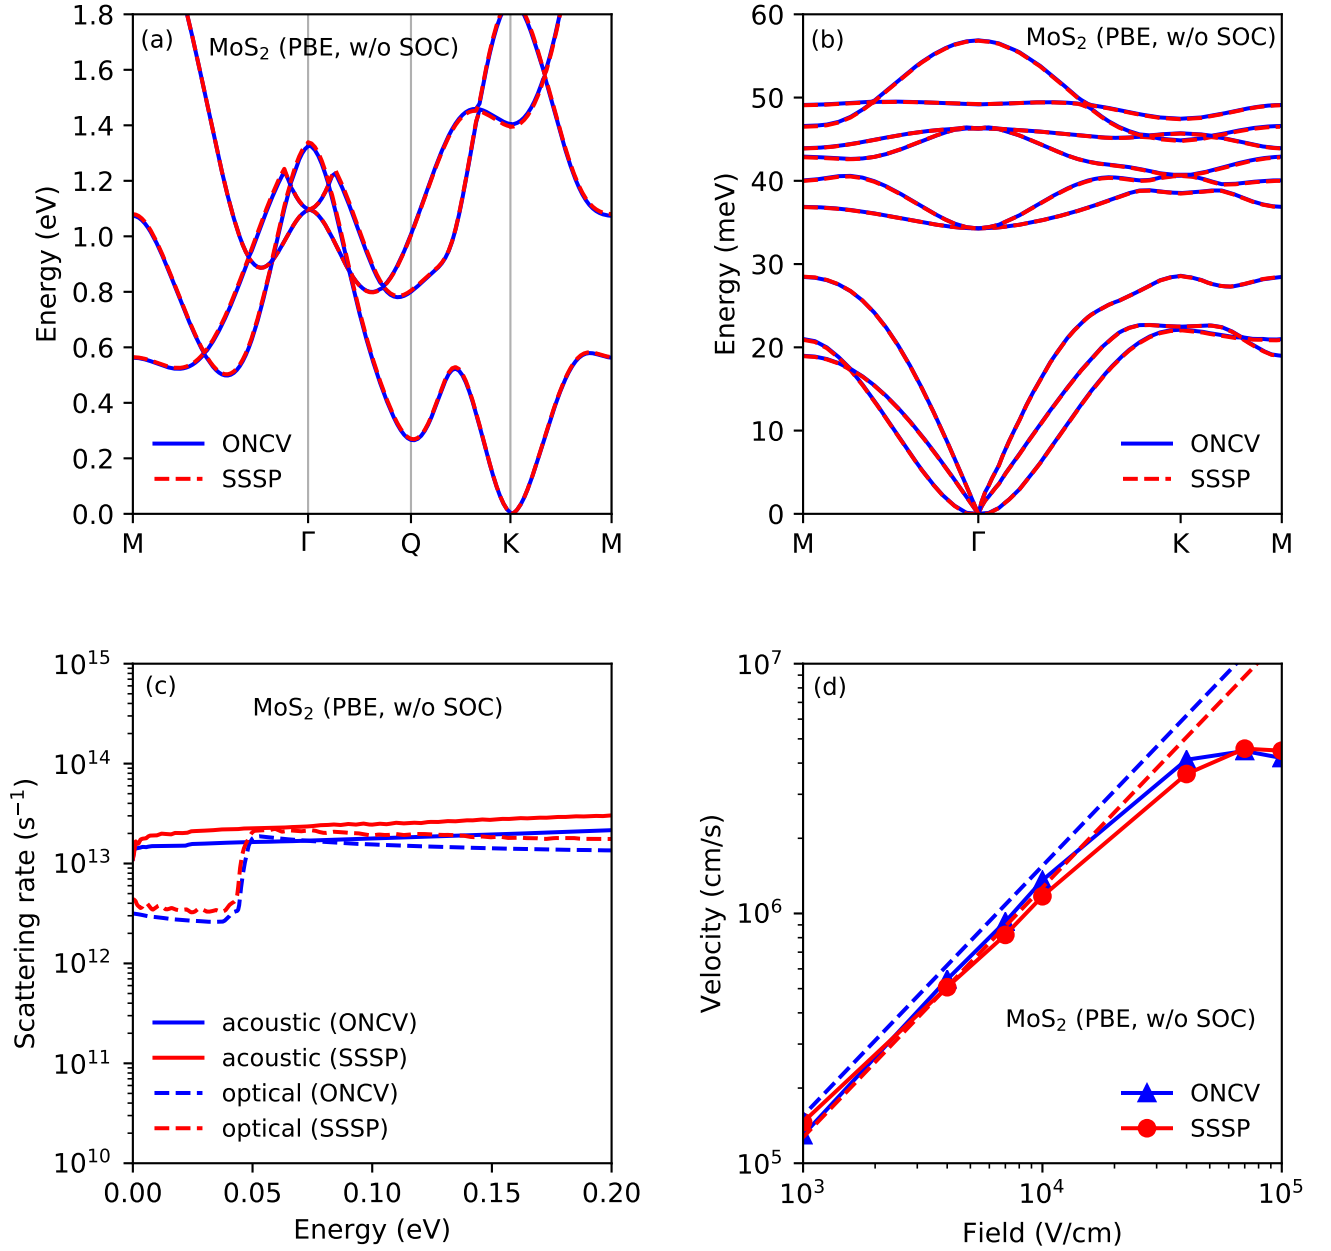

Figure S.1. (a) The electronic bandstructure, (b) phonon dispersion, (c) electron-phonon scattering rates, and (d) velocity-field characteristics for MoS<sub>2</sub>, calculated using the ONCV pseudopotentials and the SSSP for the pseudopotentials, the GGA-PBE exchange-correlation functional, and without spin-orbit coupling.

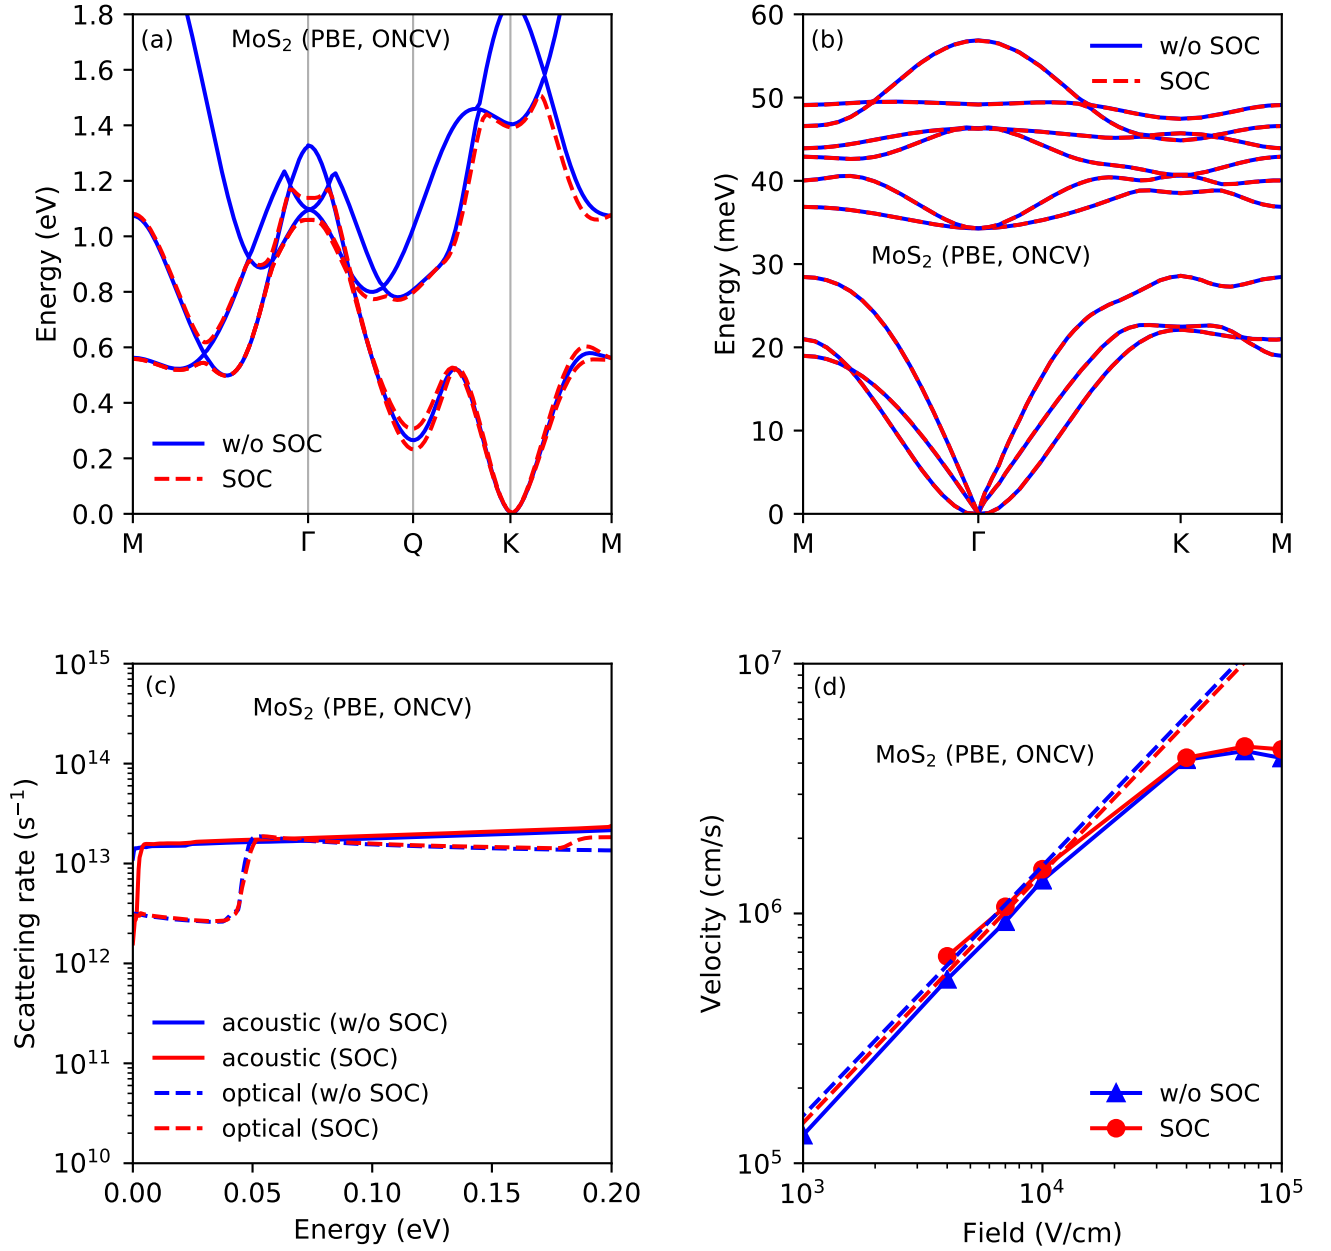

Figure S.2. (a) The electronic bandstructure, (b) phonon dispersion, (c) electron-phonon scattering rates, and (d) velocity-field characteristics for MoS<sub>2</sub>, calculated using the ONCV pseudopotentials, the GGA-PBE exchange-correlation functional, with and without spin-orbit coupling.

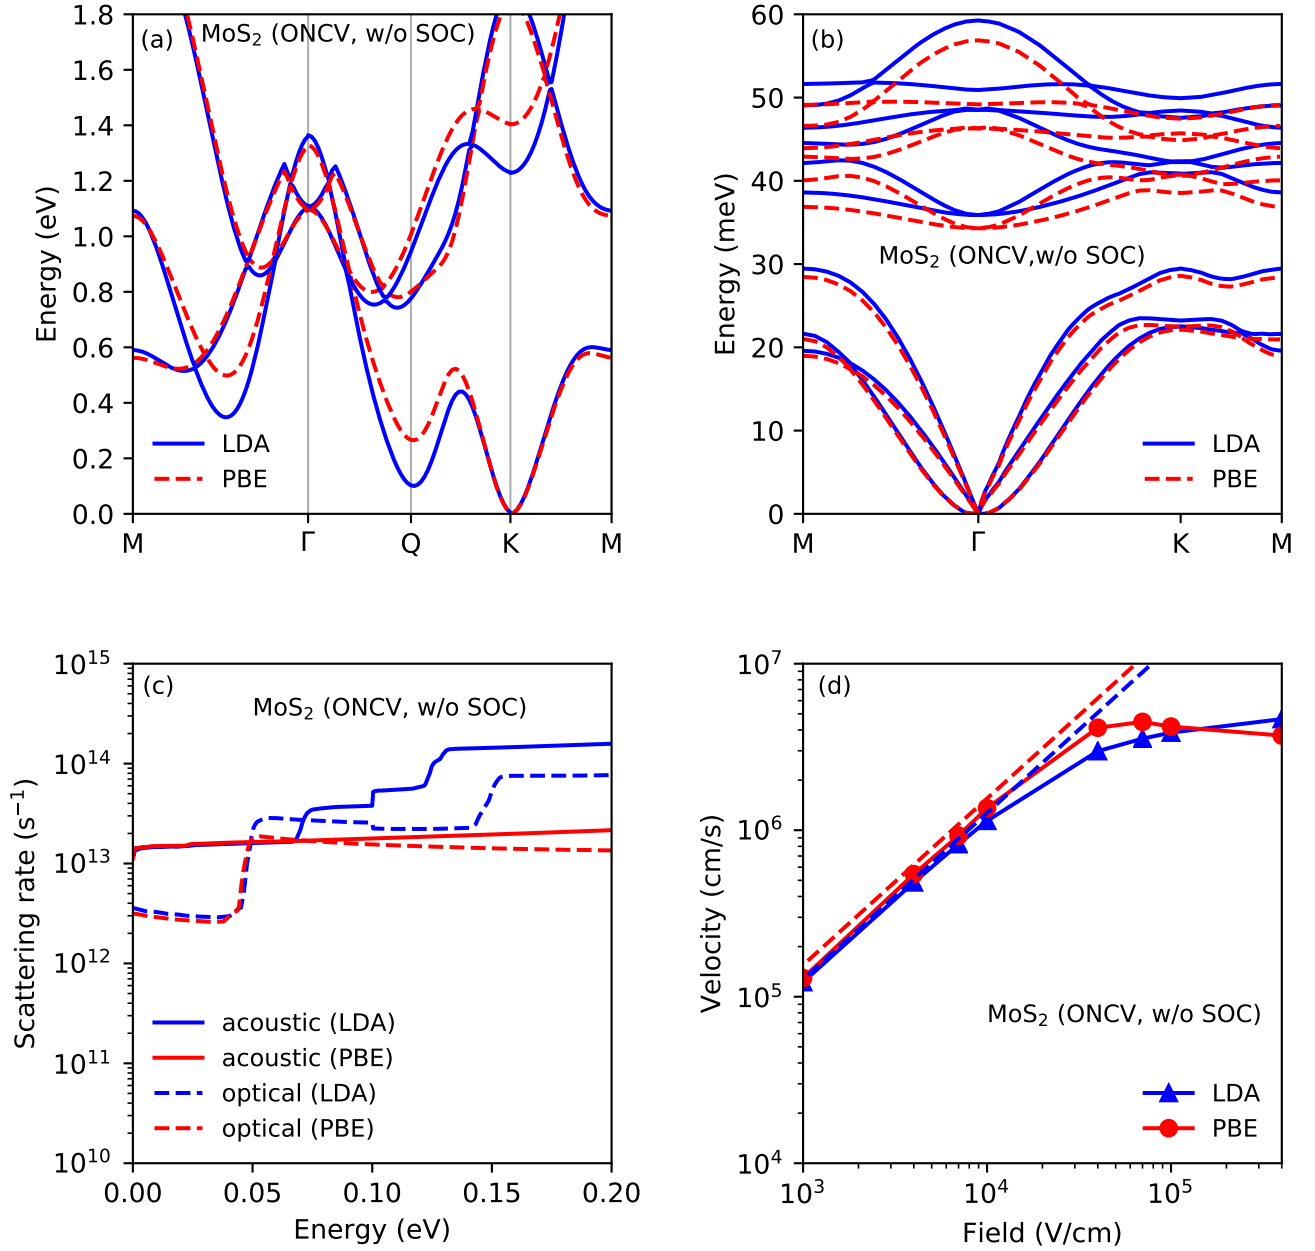

Figure S.3. (a) The electronic bandstructure, (b) phonon dispersion, (c) electron-phonon scattering rates, and (d) velocity-field characteristics for MoS<sub>2</sub>, calculated using the ONCV pseudopotentials, the LDA and the GGA-PBE exchange-correlation functional, and without spin-orbit coupling.

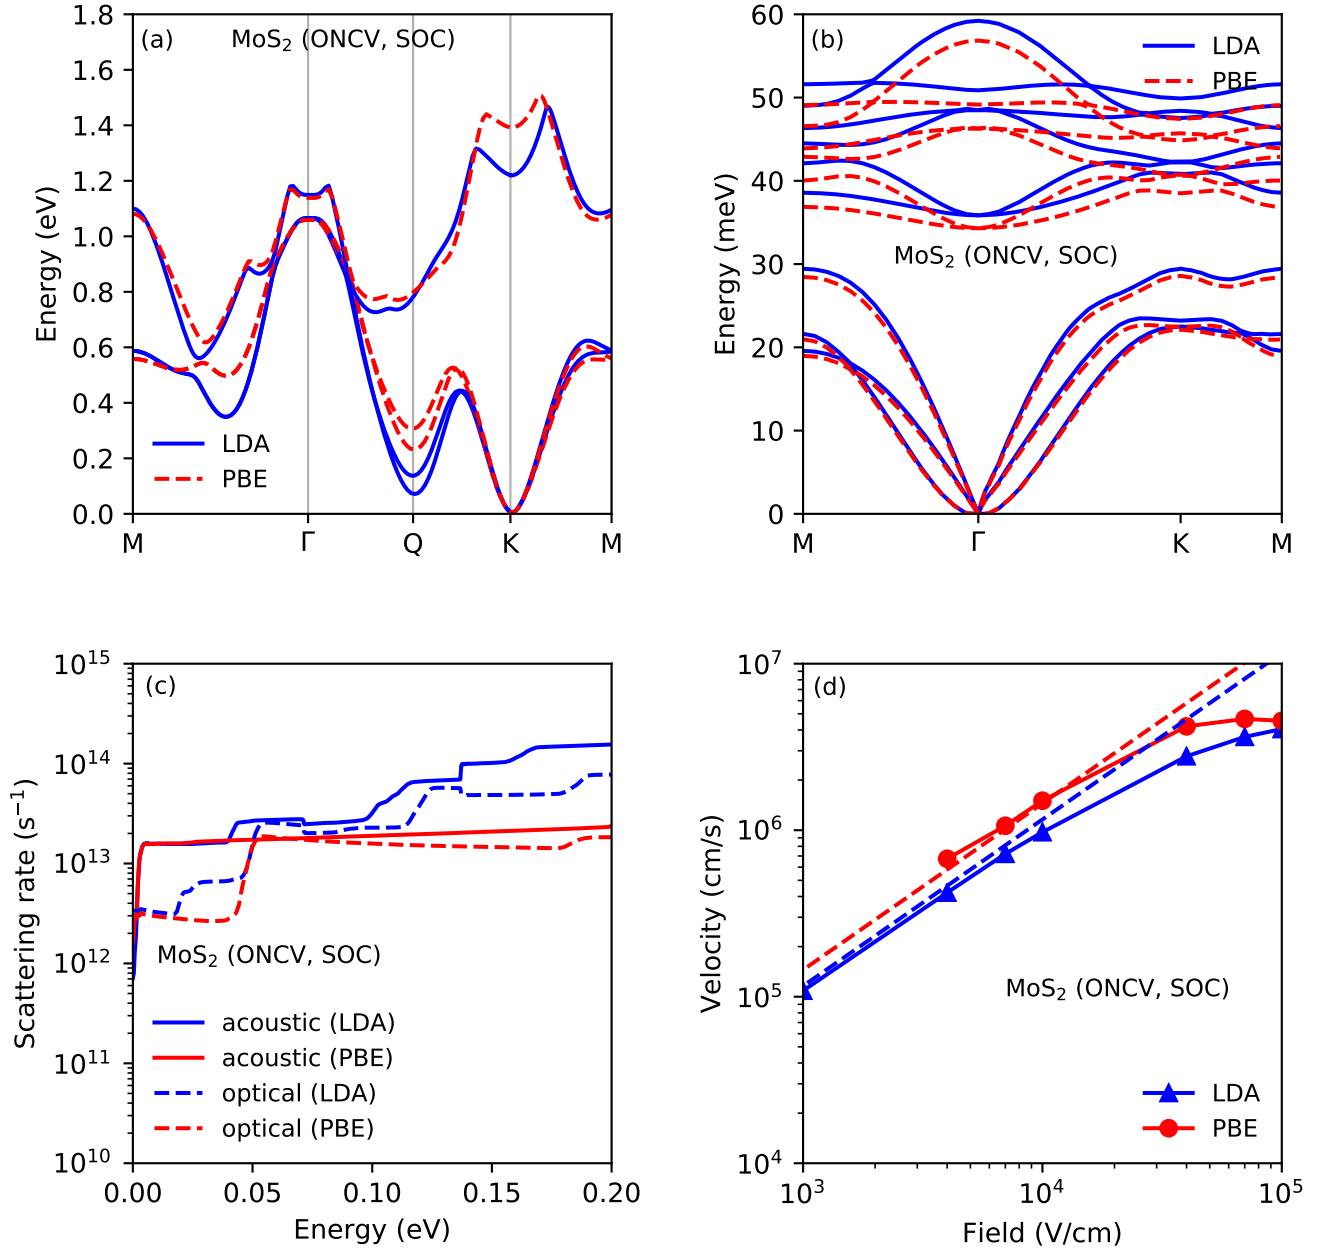

Figure S.4. (a) The electronic bandstructure, (b) phonon dispersion, (c) electron-phonon scattering rates, and (d) velocity-field characteristics for MoS<sub>2</sub>, calculated using the ONCV pseudopotentials, the LDA and the GGA-PBE exchange-correlation functional, and with spin-orbit coupling.

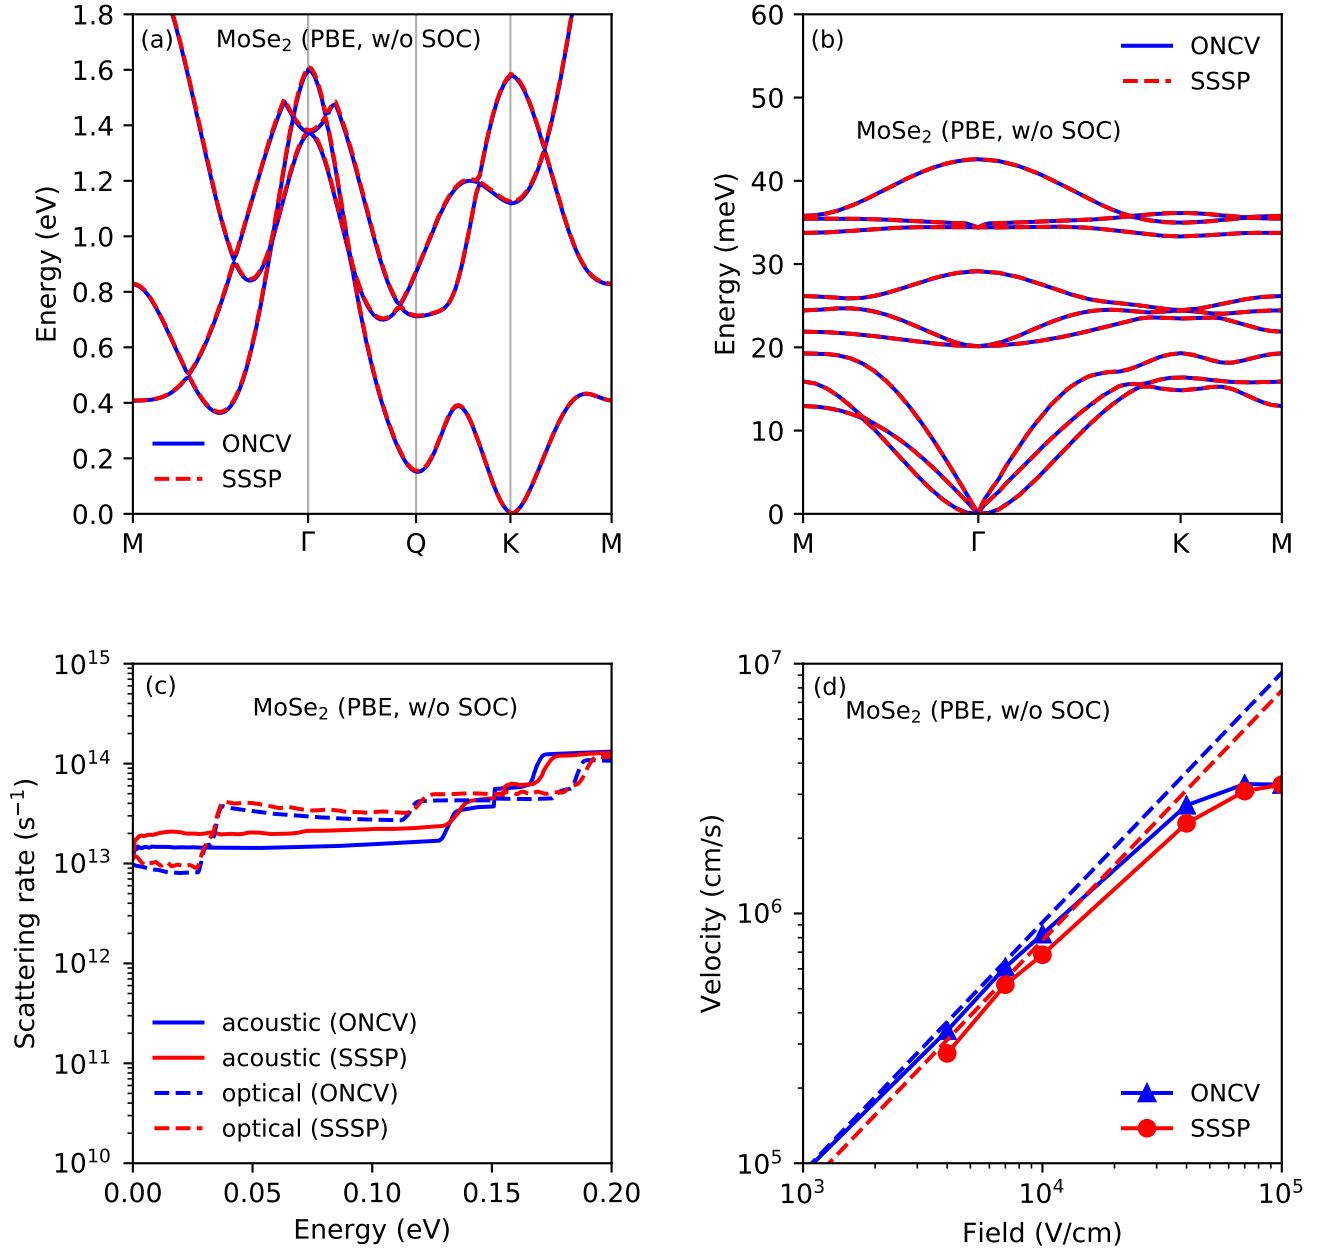

Figure S.5. (a) The electronic bandstructure, (b) phonon dispersion, (c) electron-phonon scattering rates, and (d) velocity-field characteristics for MoSe<sub>2</sub>, calculated using the ONCV pseudopotentials and the SSSP for the pseudopotentials, the GGA-PBE exchange-correlation functional, and without spin-orbit coupling.

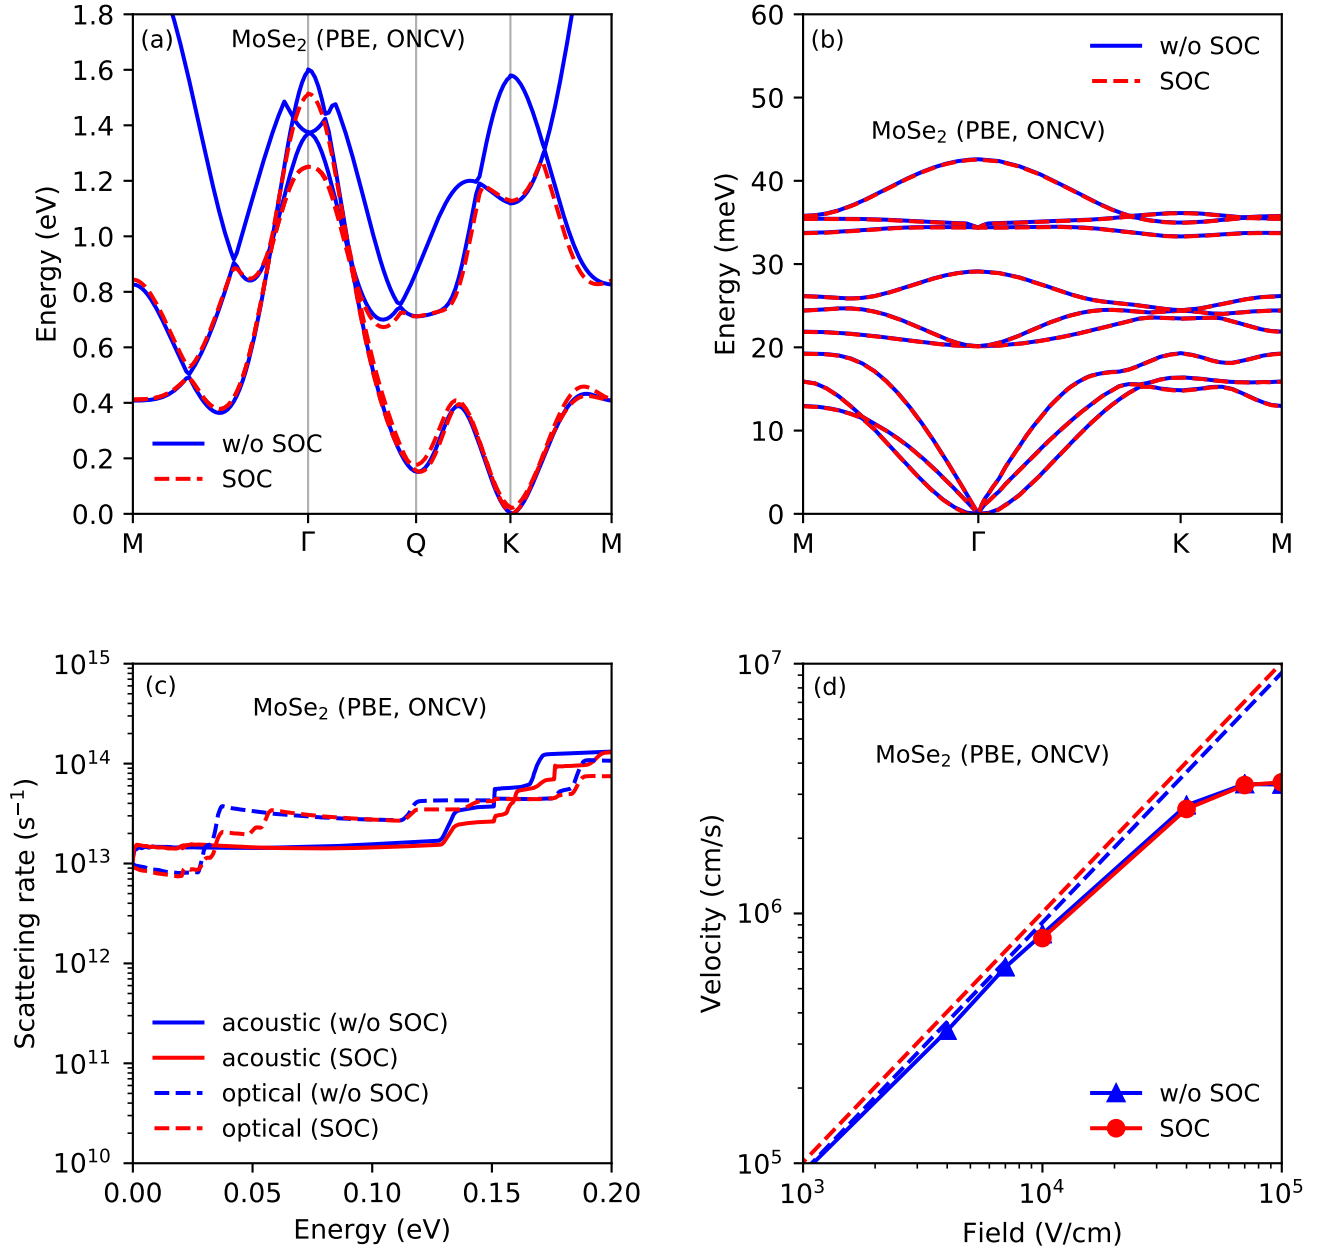

Figure S.6. (a) The electronic bandstructure, (b) phonon dispersion, (c) electron-phonon scattering rates, and (d) velocity-field characteristics for MoSe<sub>2</sub>, calculated using the ONCV pseudopotentials, the GGA-PBE exchange-correlation functional, with and without spin-orbit coupling.

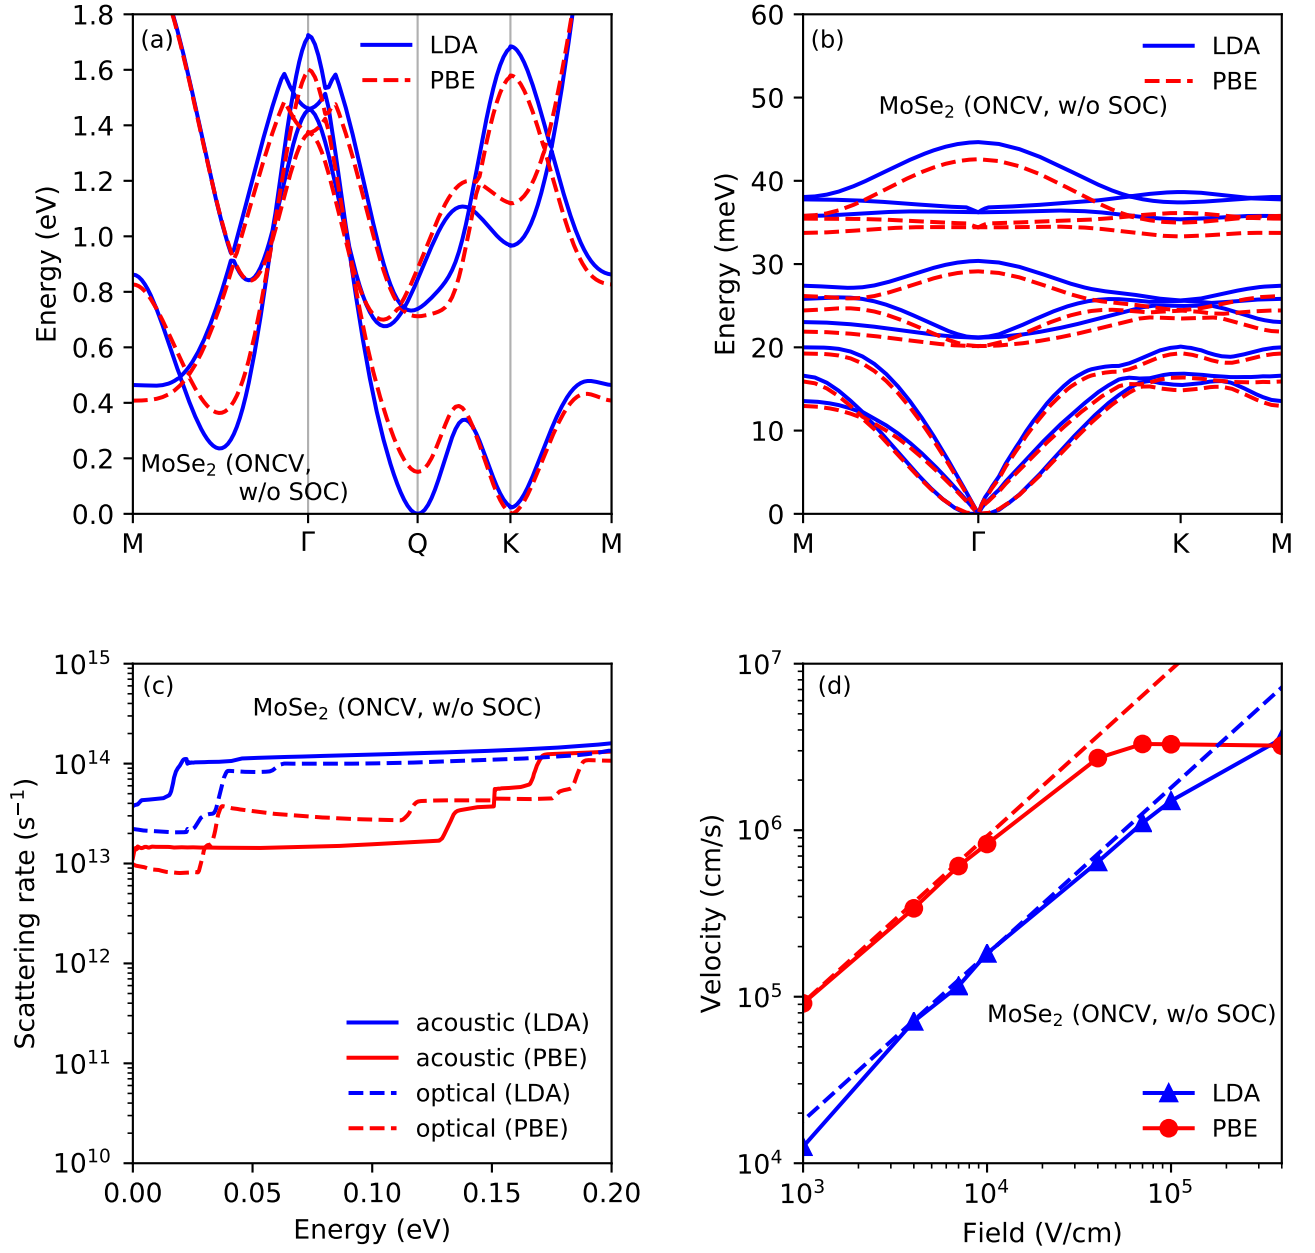

Figure S.7. (a) The electronic bandstructure, (b) phonon dispersion, (c) electron-phonon scattering rates, and (d) velocity-field characteristics for MoSe<sub>2</sub>, calculated using the ONCV pseudopotentials, the LDA and the GGA-PBE exchange-correlation functional, and without spin-orbit coupling.



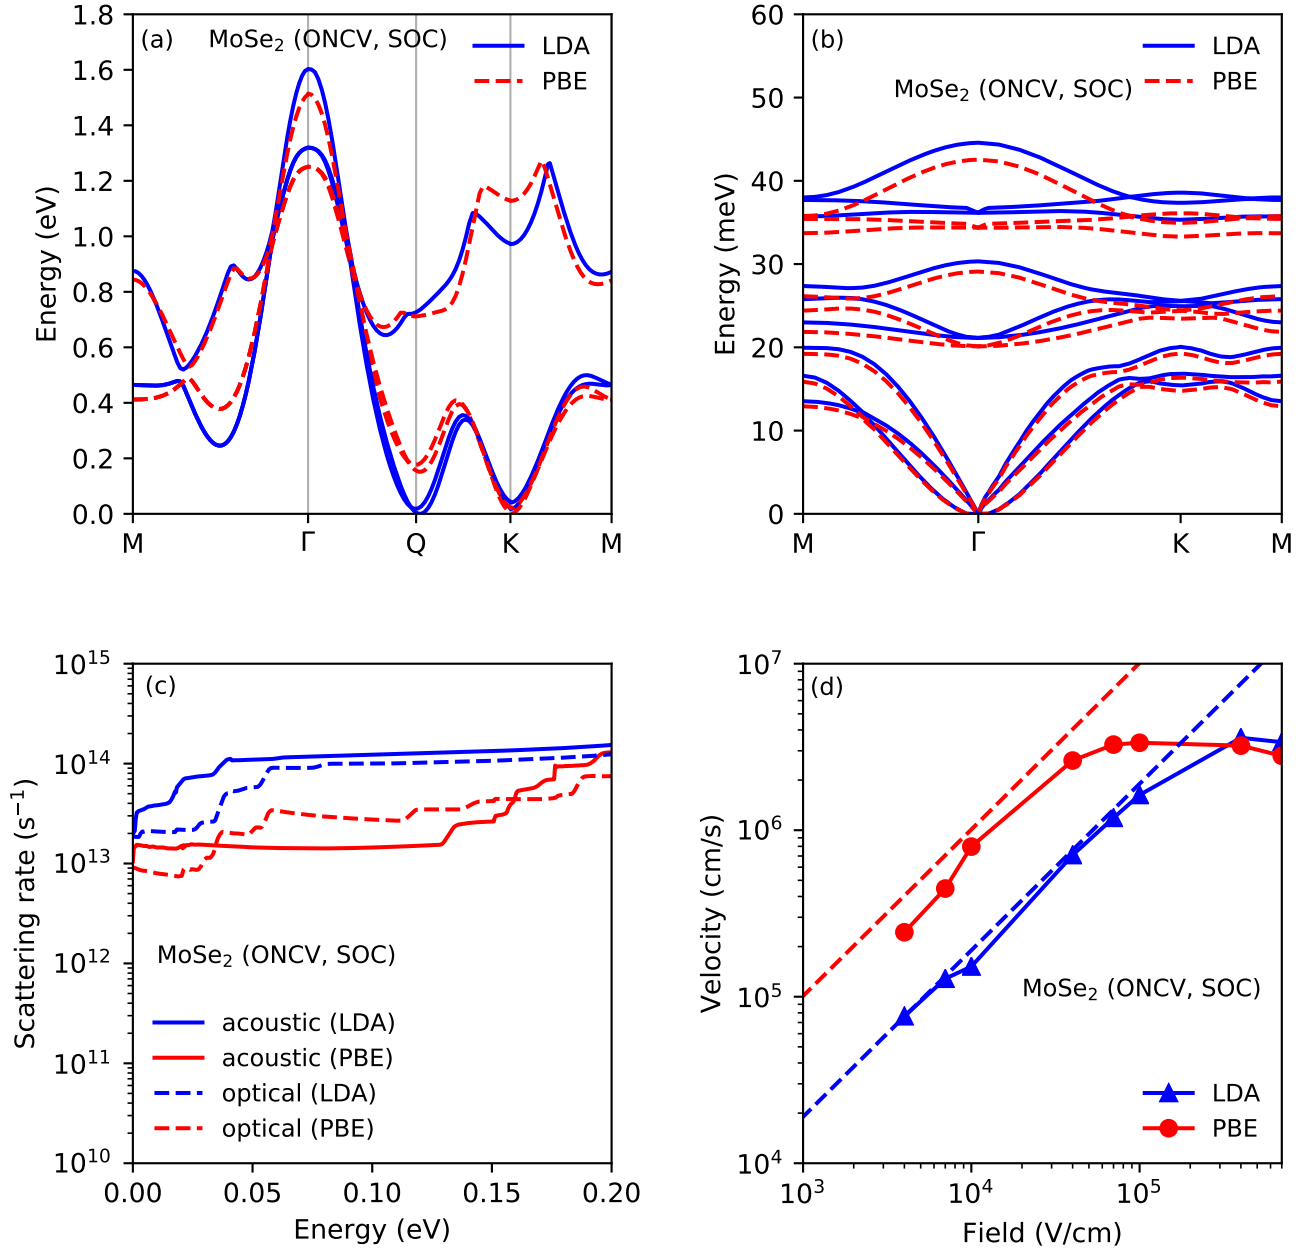

Figure S.8. (a) The electronic bandstructure, (b) phonon dispersion, (c) electron-phonon scattering rates, and (d) velocity-field characteristics for MoSe<sub>2</sub>, calculated using the ONCV pseudopotentials, the LDA and the GGA-PBE exchange-correlation functional, and with spin-orbit coupling.

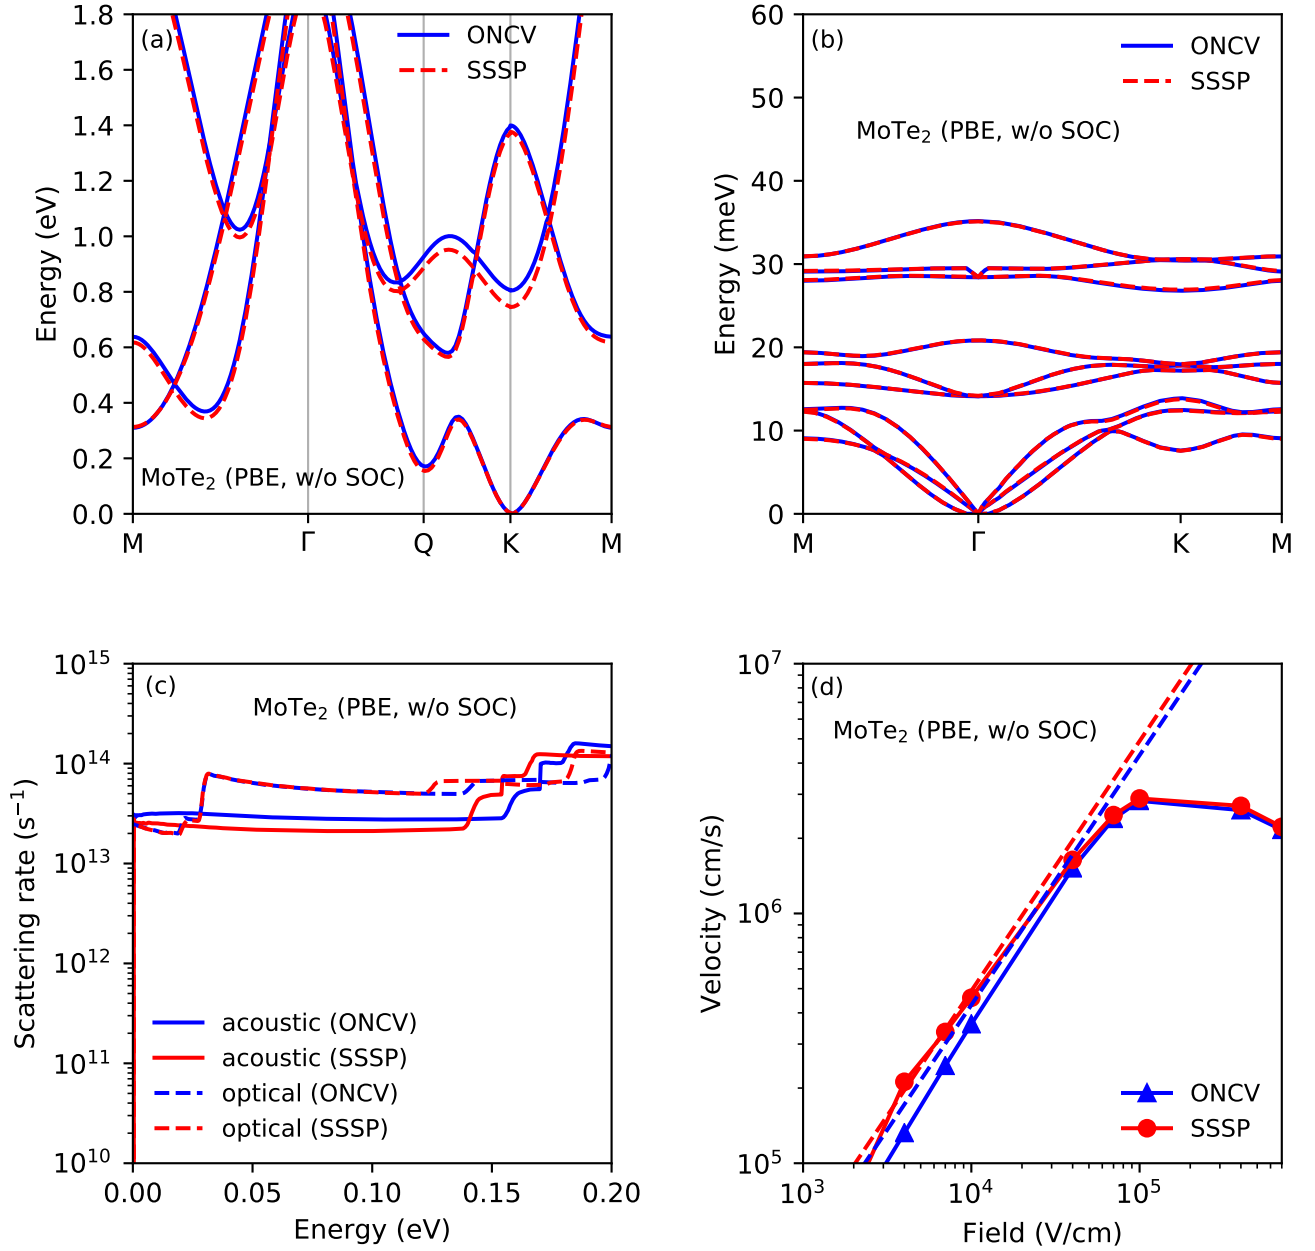

Figure S.9. (a) The electronic bandstructure, (b) phonon dispersion, (c) electron-phonon scattering rates, and (d) velocity-field characteristics for MoTe<sub>2</sub>, calculated using the ONCV pseudopotentials and the SSSP for the pseudopotentials, the GGA-PBE exchange-correlation functional, and without spin-orbit coupling.

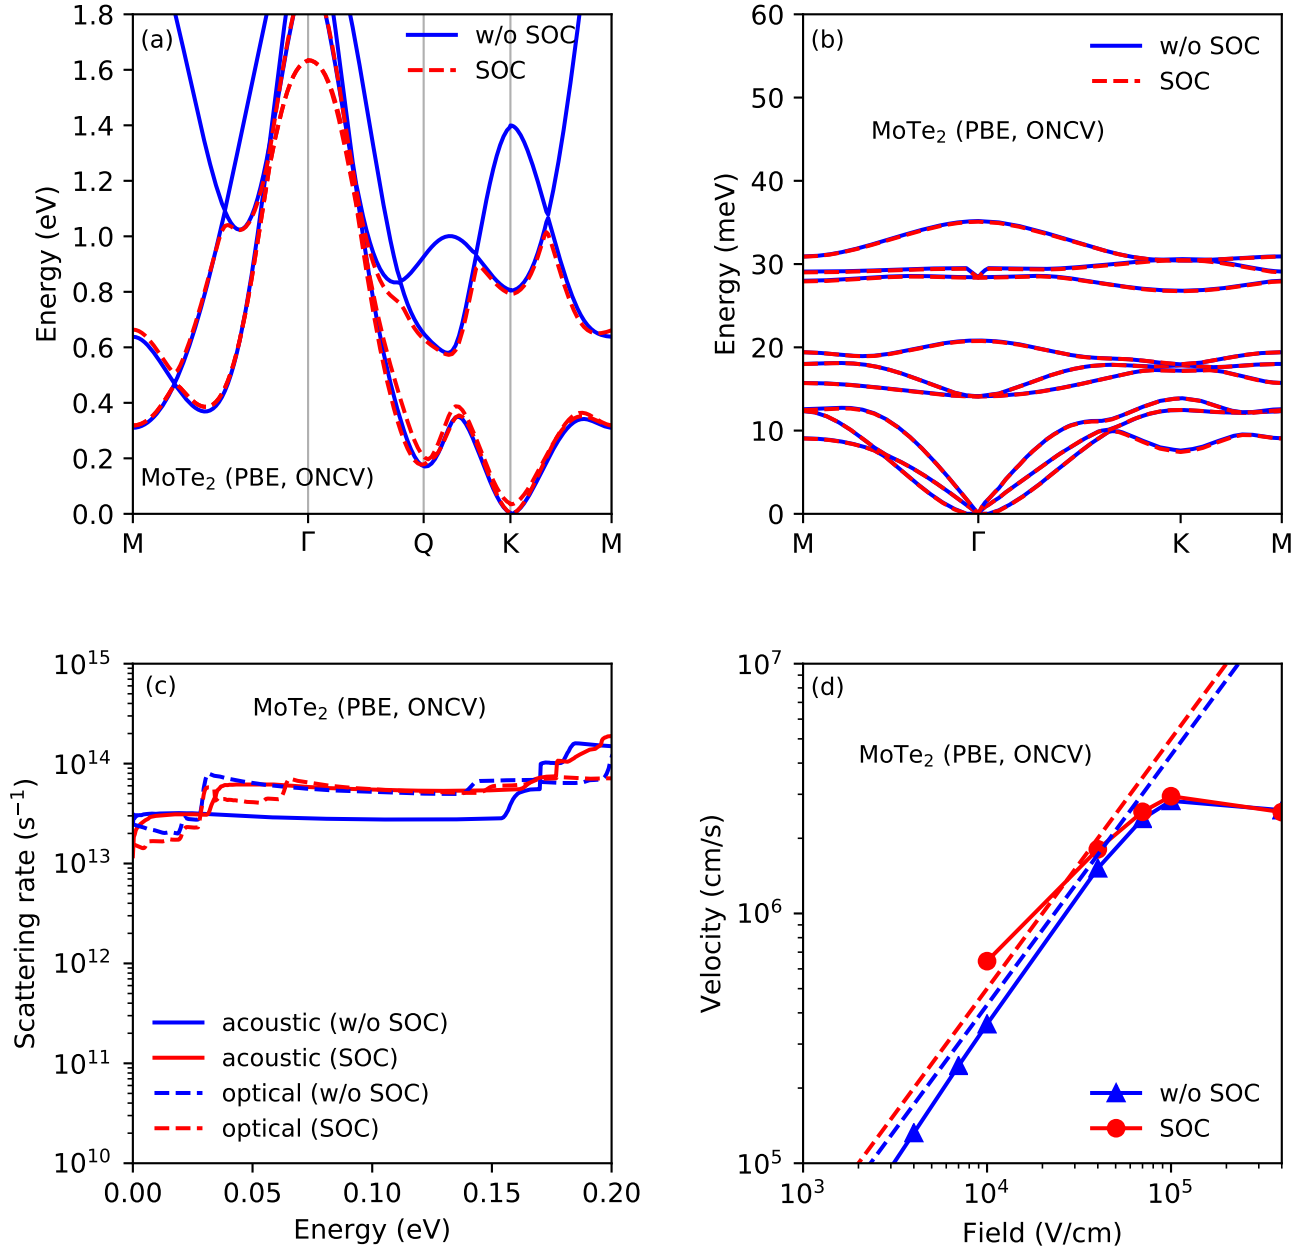

Figure S.10. (a) The electronic bandstructure, (b) phonon dispersion, (c) electron-phonon scattering rates, and (d) velocity-field characteristics for MoTe<sub>2</sub>, calculated using the ONCV pseudopotentials, the GGA-PBE exchange-correlation functional, with and without spin-orbit coupling.

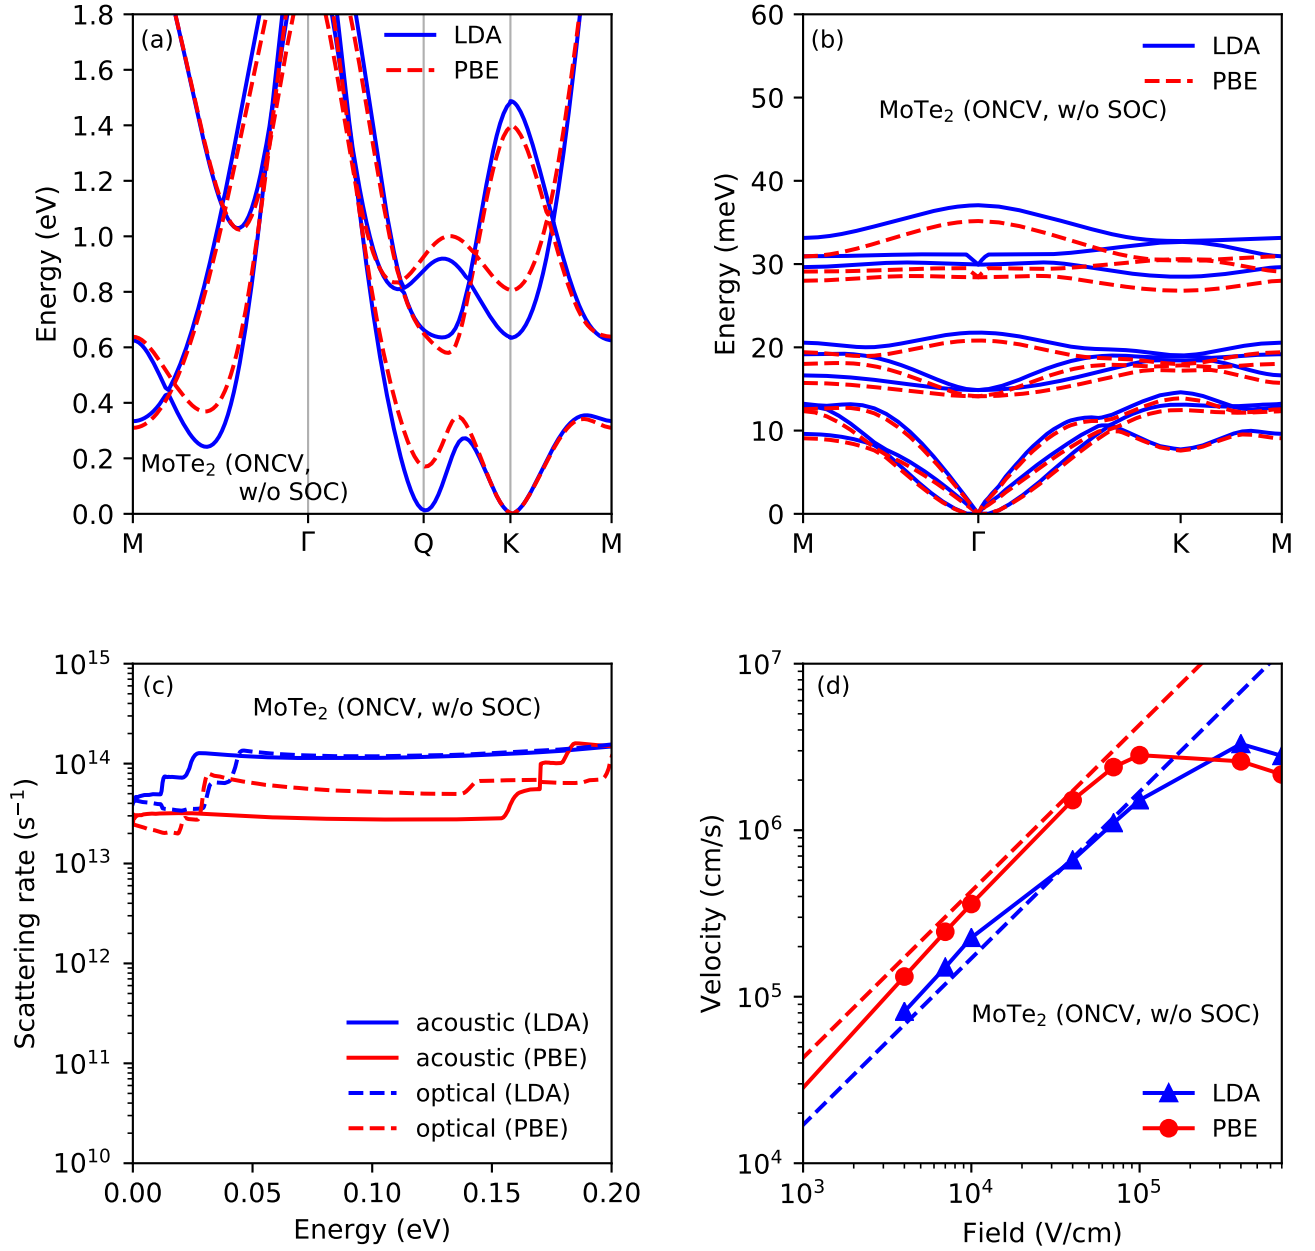

Figure S.11. (a) The electronic bandstructure, (b) phonon dispersion, (c) electron-phonon scattering rates, and (d) velocity-field characteristics for  $\text{MoTe}_2$ , calculated using the ONCV pseudopotentials, the LDA and the GGA-PBE exchange-correlation functional, and without spin-orbit coupling.

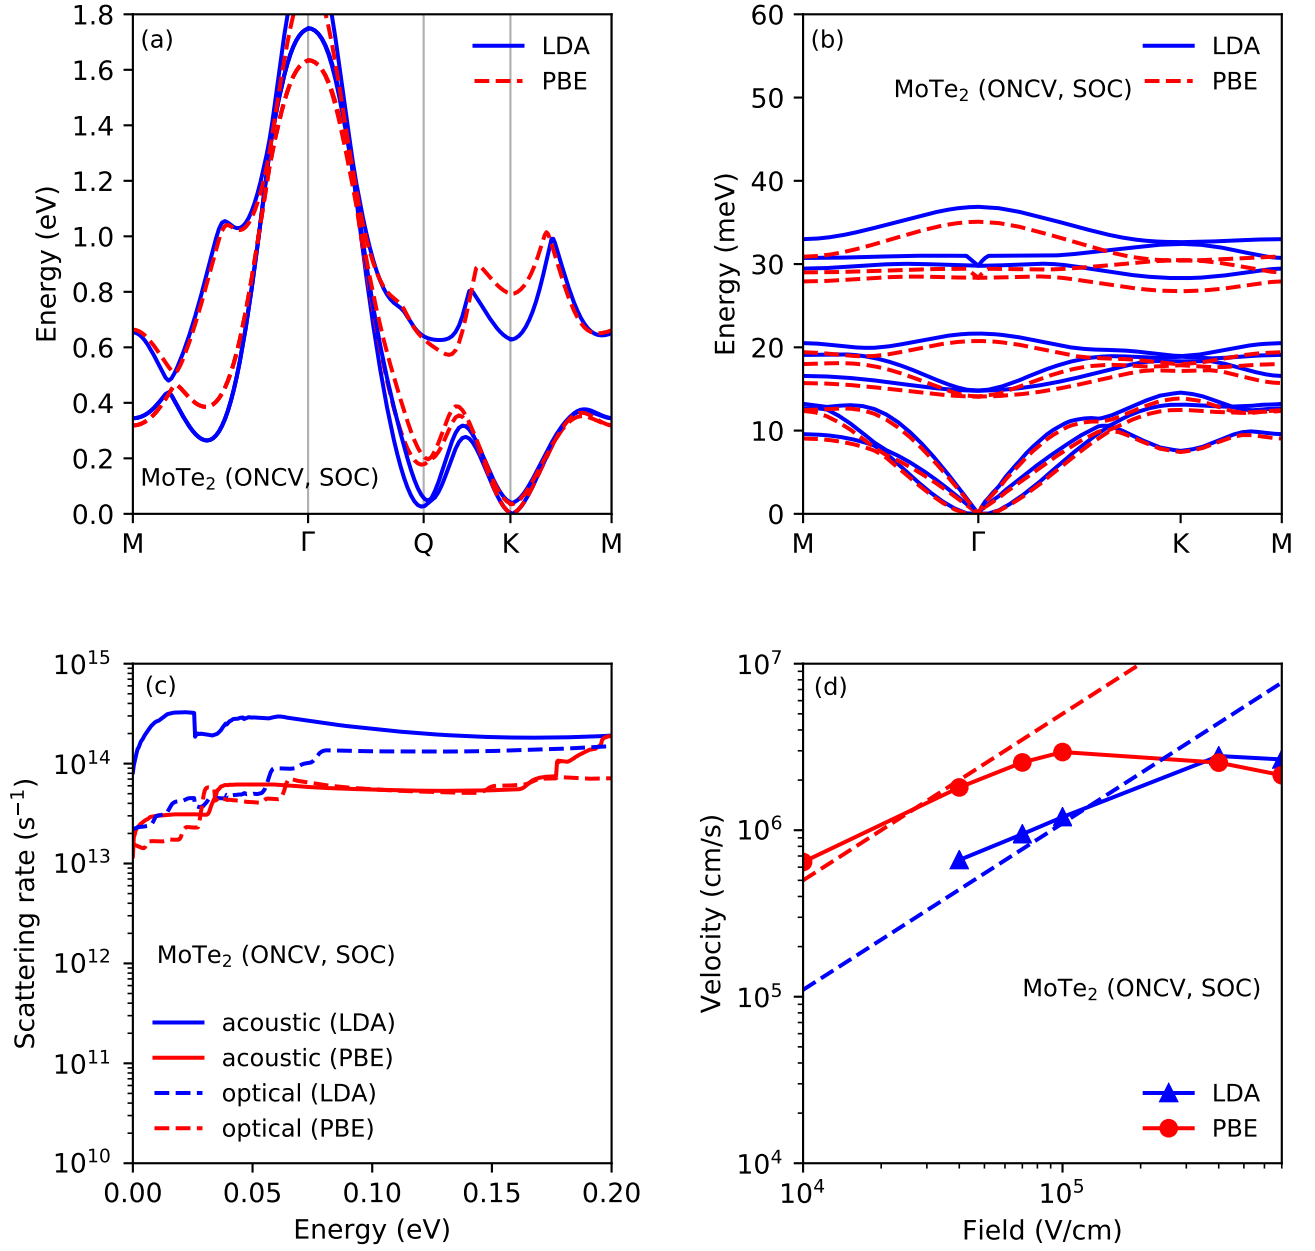

Figure S.12. (a) The electronic bandstructure, (b) phonon dispersion, (c) electron-phonon scattering rates, and (d) velocity-field characteristics for MoTe<sub>2</sub>, calculated using the ONCV pseudopotentials, the LDA and the GGA-PBE exchange-correlation functional, and with spin-orbit coupling.

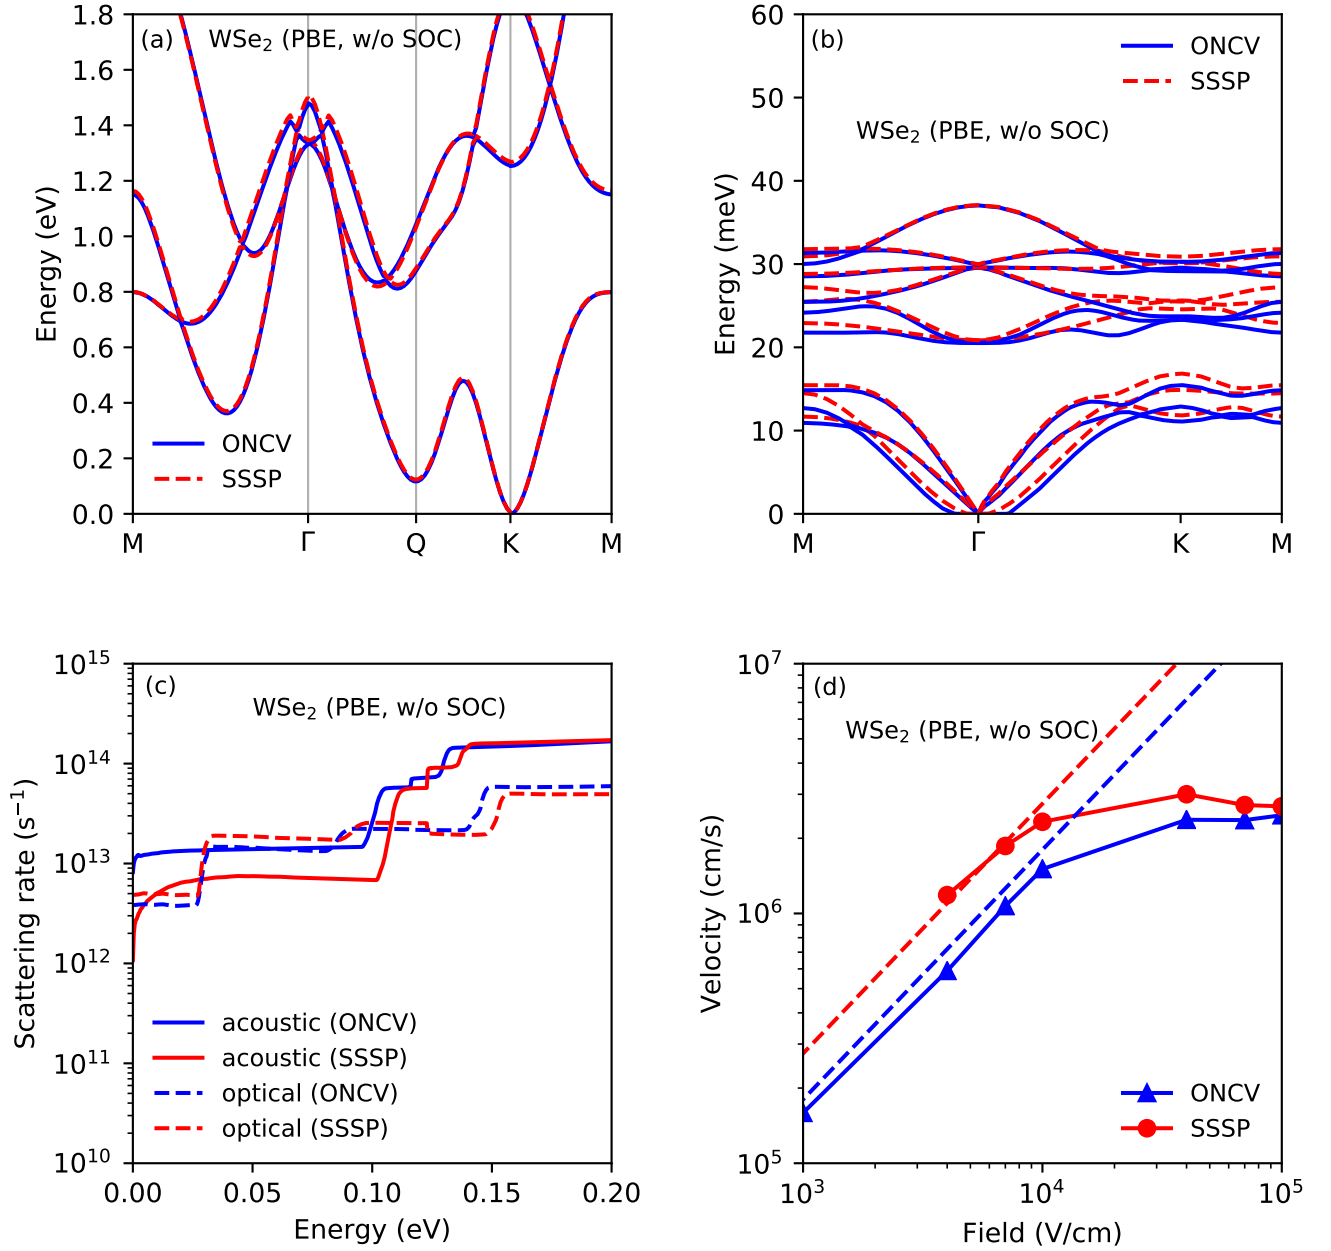

Figure S.13. (a) The electronic bandstructure, (b) phonon dispersion, (c) electron-phonon scattering rates, and (d) velocity-field characteristics for  $\text{WSe}_2$ , calculated using the ONCV pseudopotentials and the SSSP for the pseudopotentials, the GGA-PBE exchange-correlation functional, and without spin-orbit coupling.

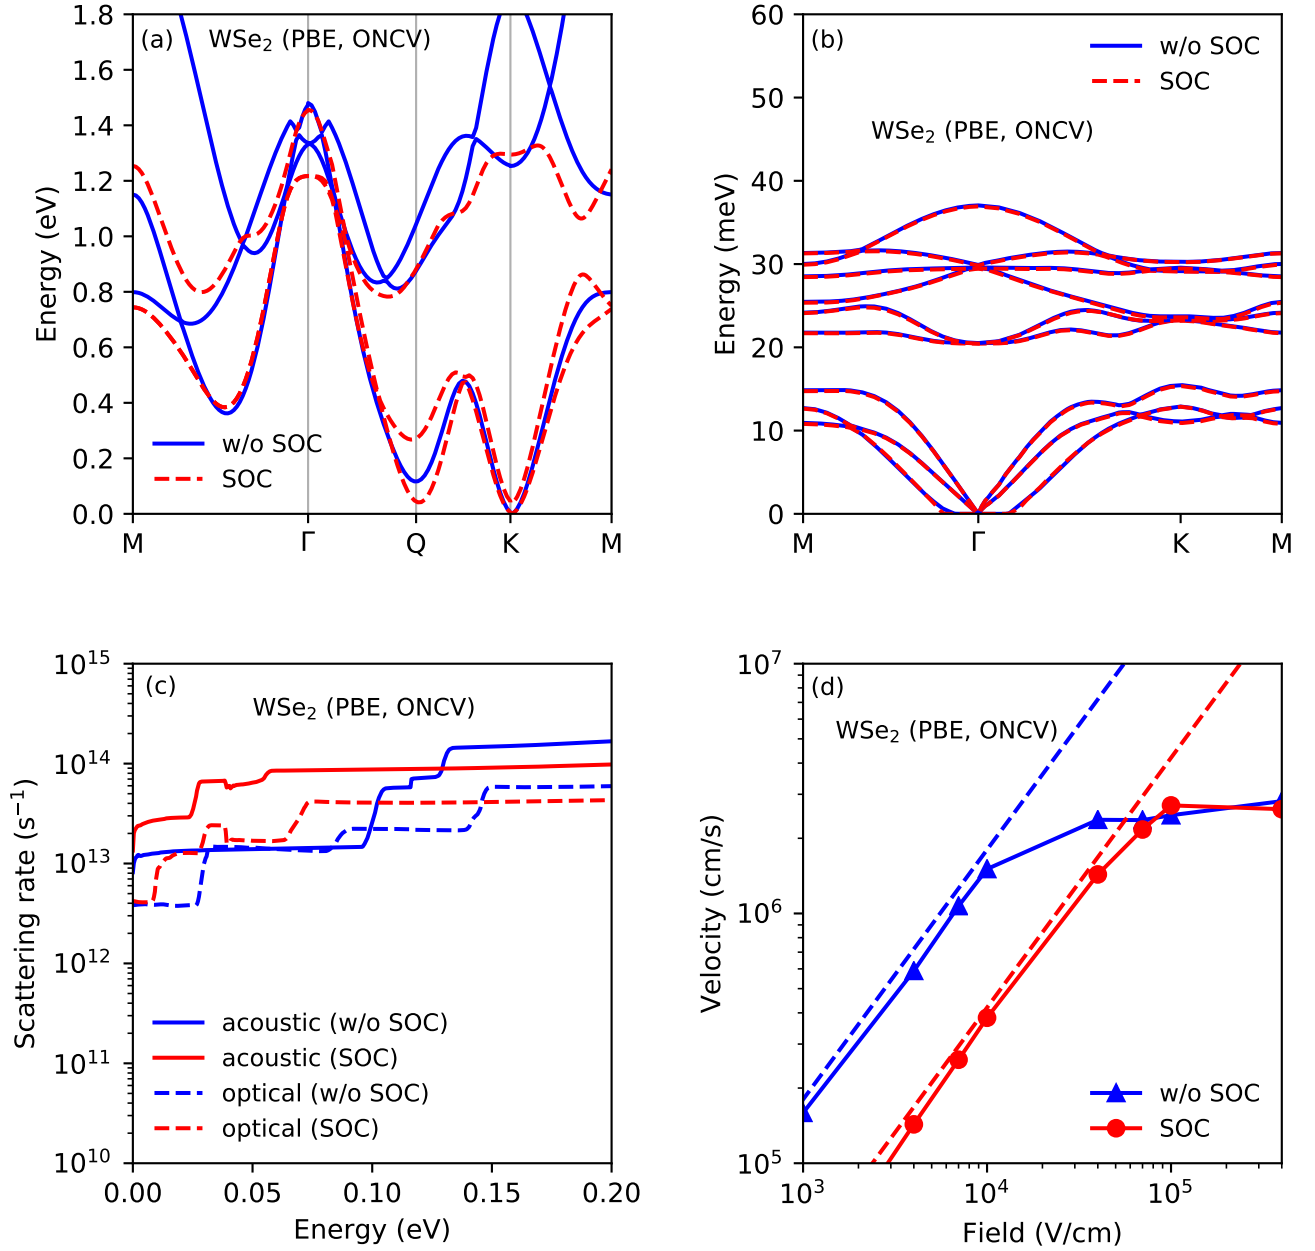

Figure S.14. (a) The electronic bandstructure, (b) phonon dispersion, (c) electron-phonon scattering rates, and (d) velocity-field characteristics for  $\text{WSe}_2$ , calculated using the ONCV pseudopotentials, the GGA-PBE exchange-correlation functional, with and without spin-orbit coupling.

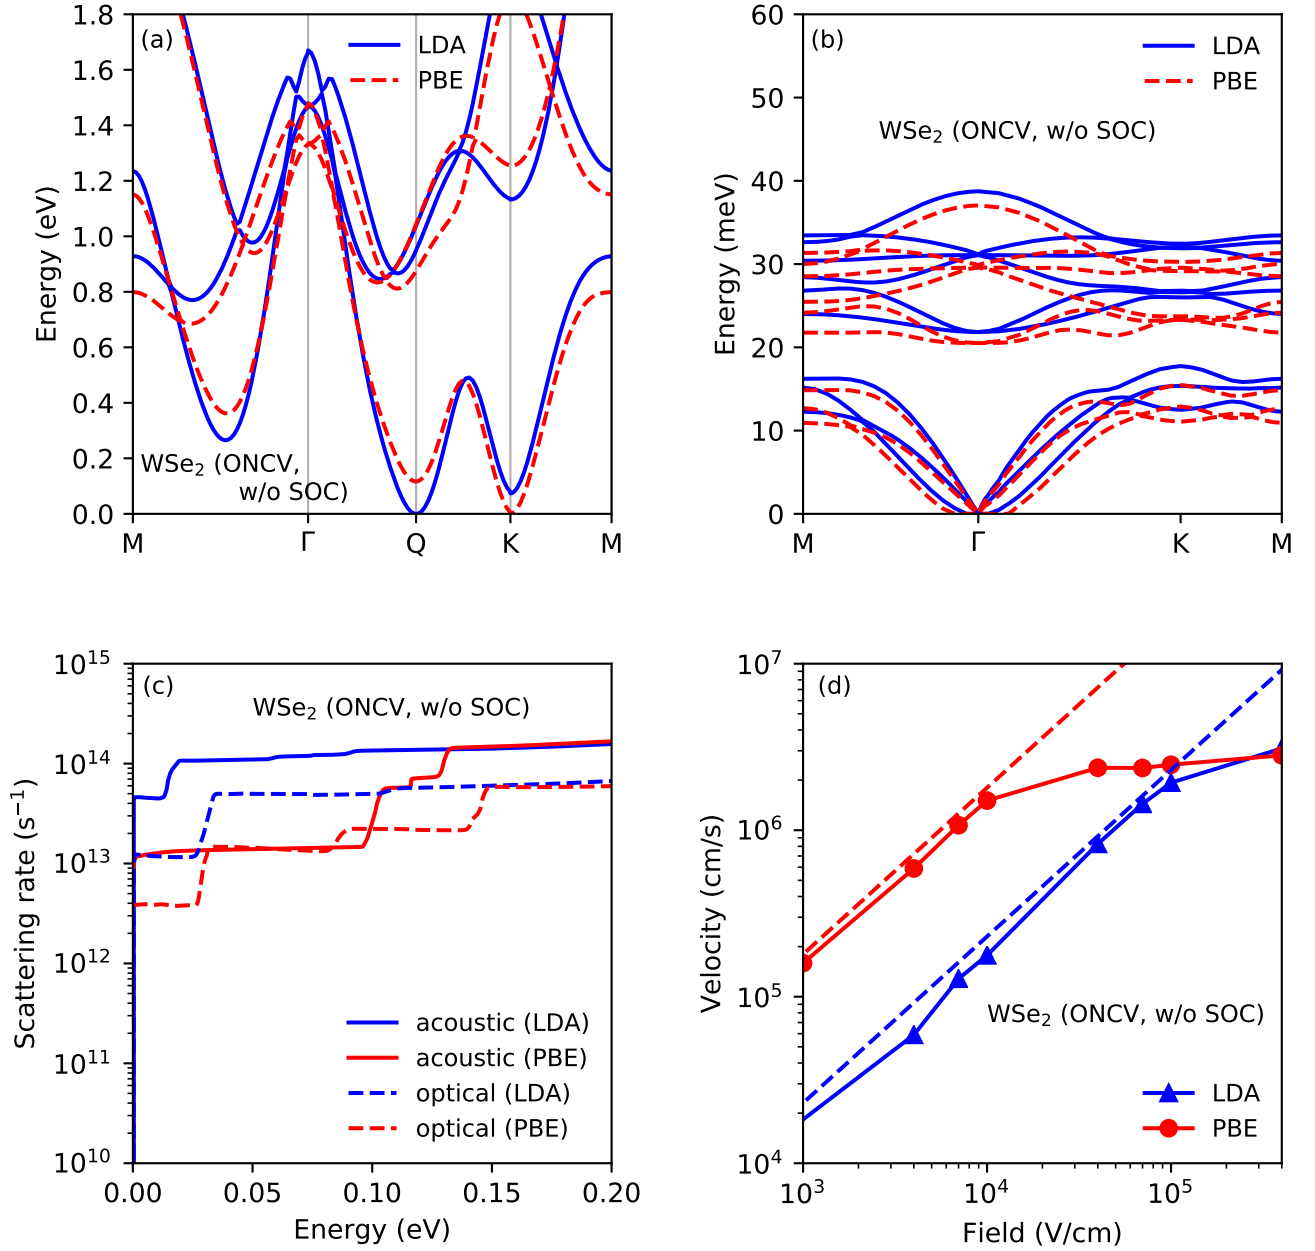

Figure S.15. (a) The electronic bandstructure, (b) phonon dispersion, (c) electron-phonon scattering rates, and (d) velocity-field characteristics for  $\text{WSe}_2$ , calculated using the ONCV pseudopotentials, the LDA and the GGA-PBE exchange-correlation functional, and without spin-orbit coupling.



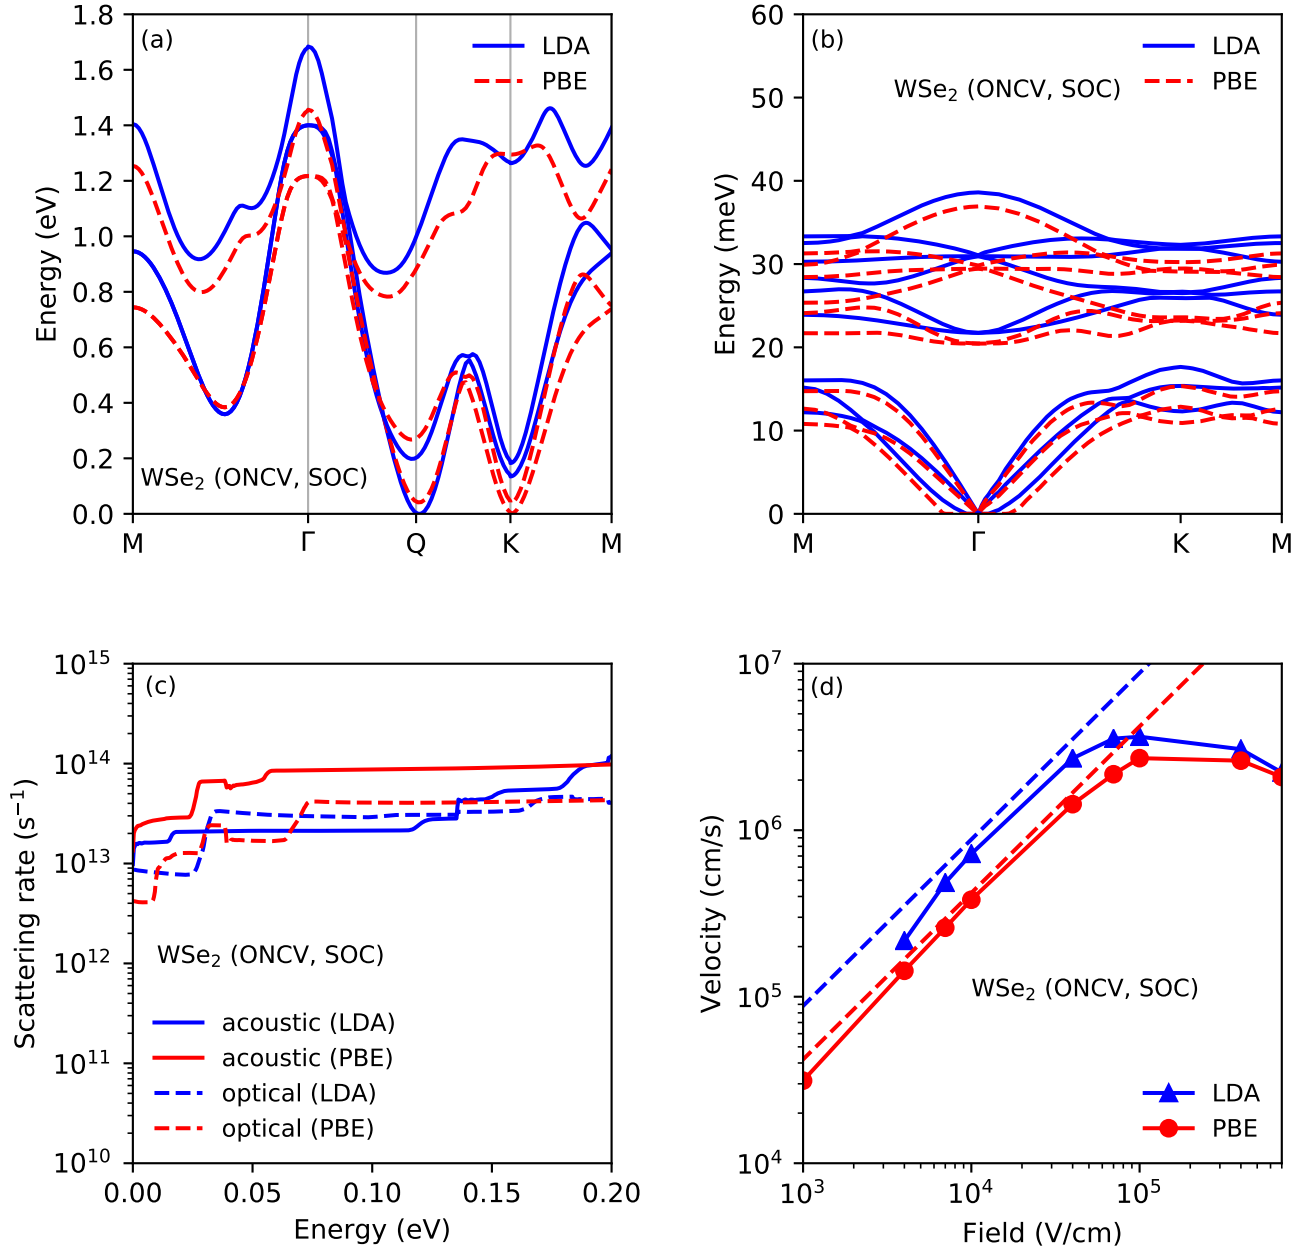

Figure S.16. (a) The electronic bandstructure, (b) phonon dispersion, (c) electron-phonon scattering rates, and (d) velocity-field characteristics for  $\text{WSe}_2$ , calculated using the ONCV pseudopotentials, the LDA and the GGA-PBE exchange-correlation functional, and with spin-orbit coupling.

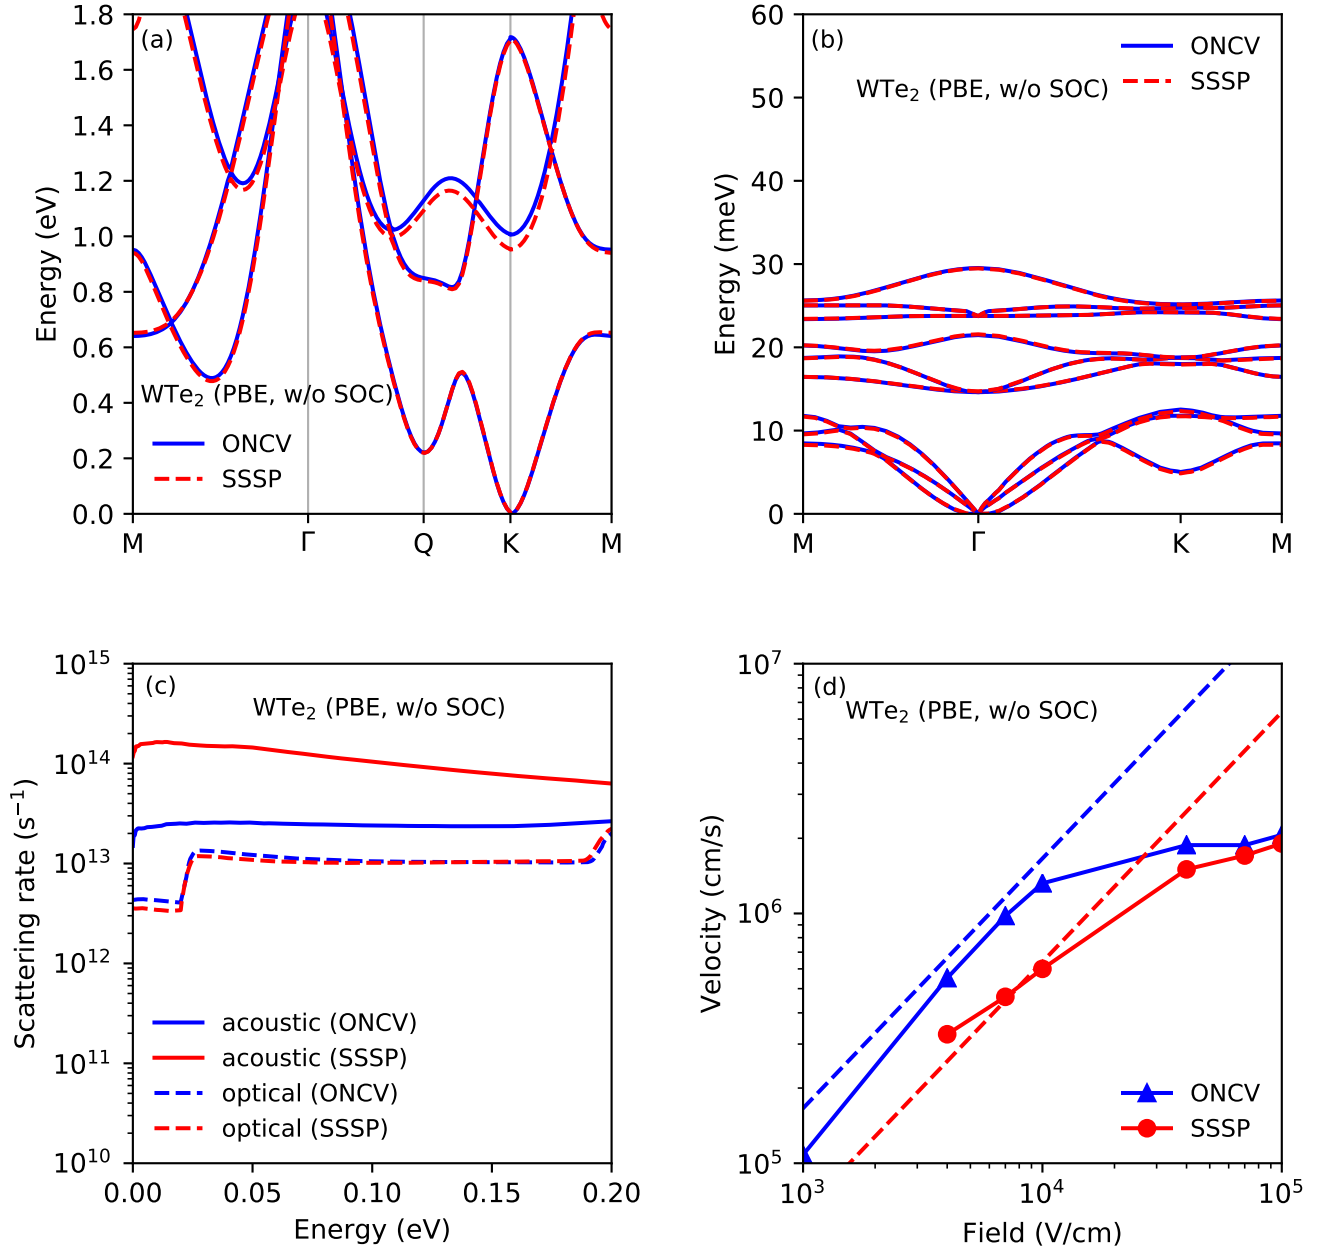

Figure S.17. (a) The electronic bandstructure, (b) phonon dispersion, (c) electron-phonon scattering rates, and (d) velocity-field characteristics for  $\text{WTe}_2$ , calculated using the ONCV pseudopotentials and the SSSP for the pseudopotentials, the GGA-PBE exchange-correlation functional, and without spin-orbit coupling.

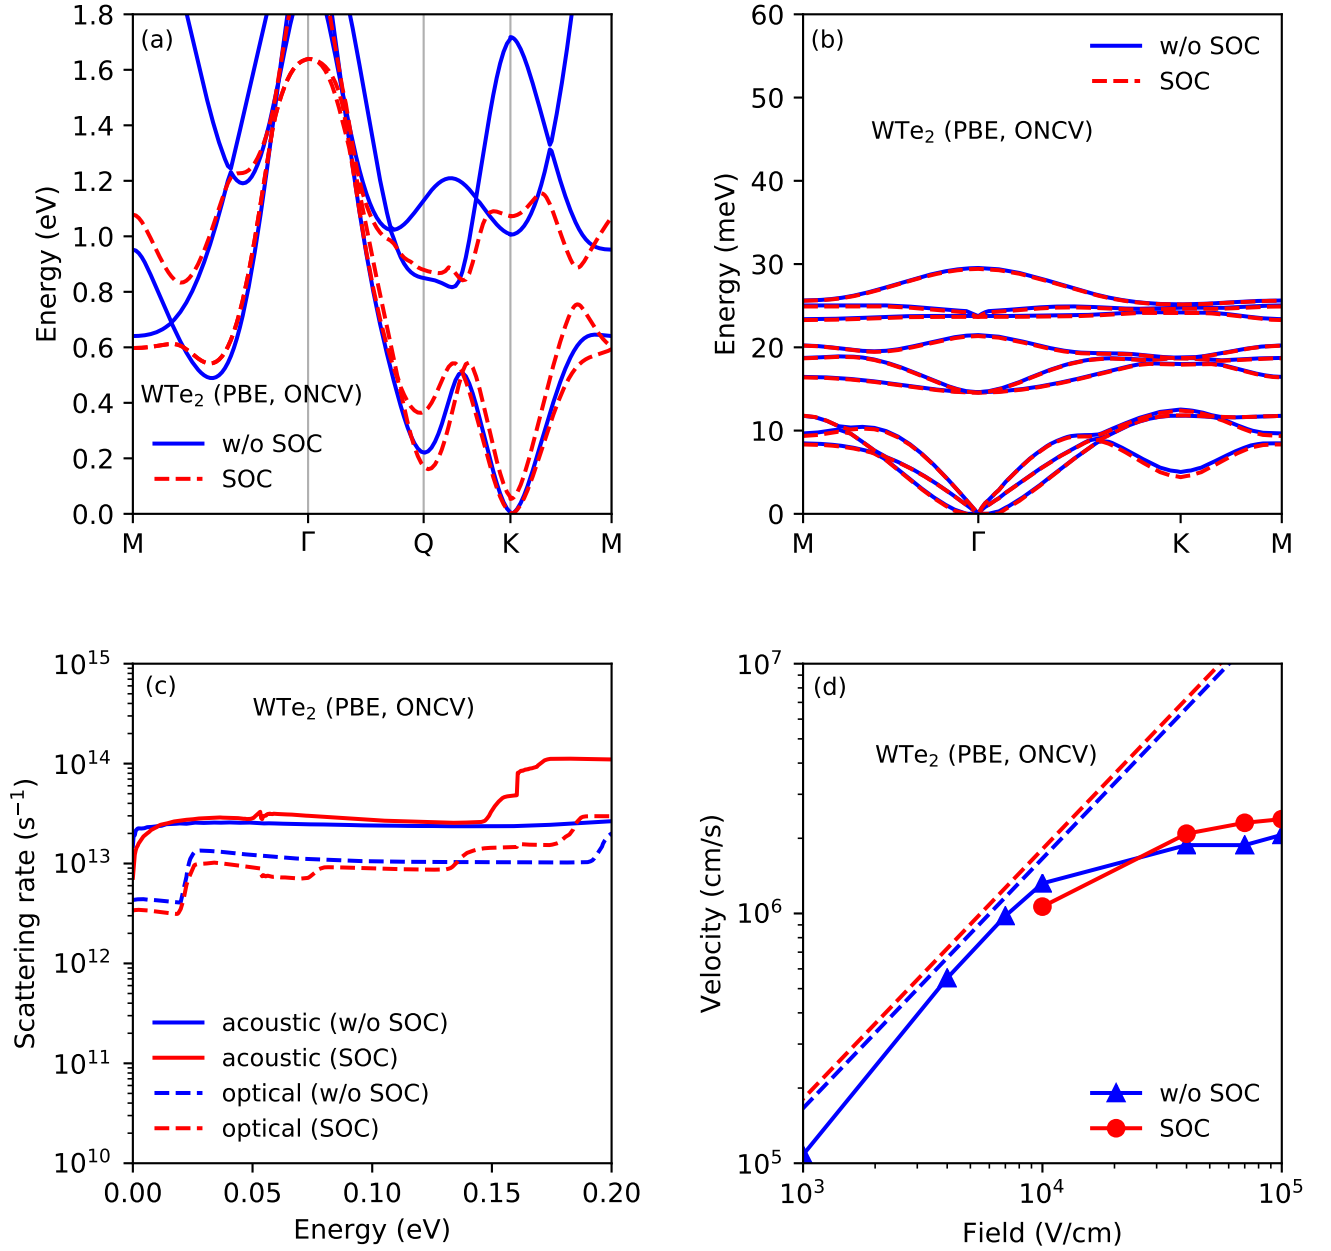

Figure S.18. (a) The electronic bandstructure, (b) phonon dispersion, (c) electron-phonon scattering rates, and (d) velocity-field characteristics for  $\text{WTe}_2$ , calculated using the ONCV pseudopotentials, the GGA-PBE exchange-correlation functional, with and without spin-orbit coupling.

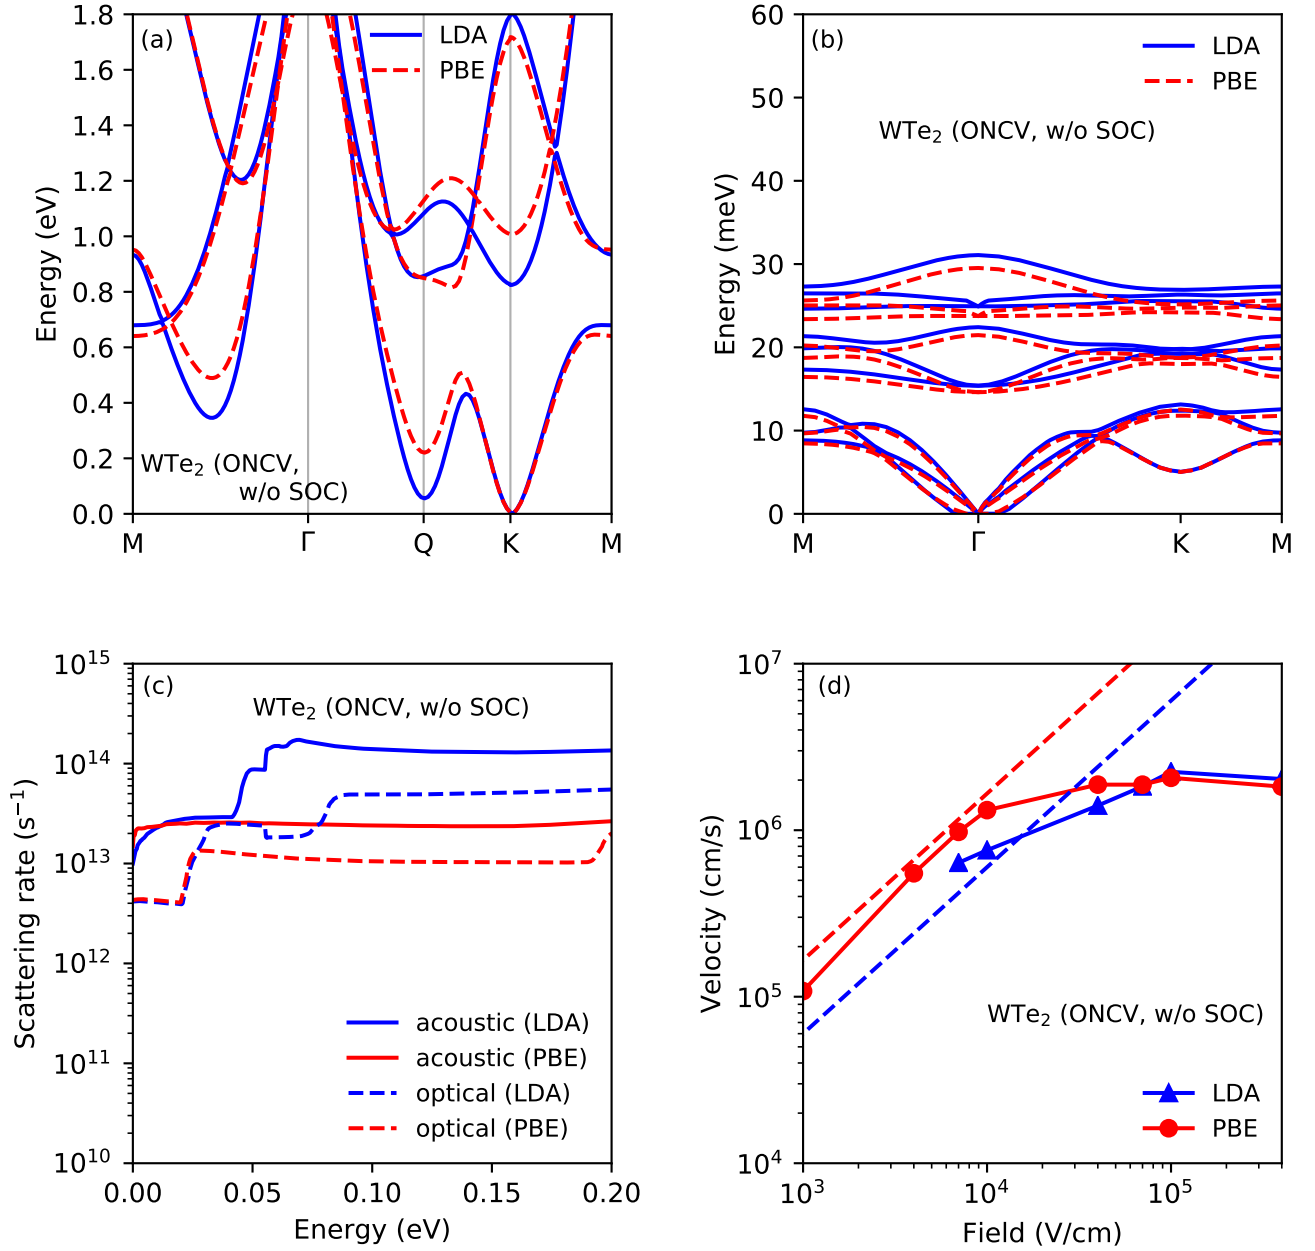

Figure S.19. (a) The electronic bandstructure, (b) phonon dispersion, (c) electron-phonon scattering rates, and (d) velocity-field characteristics for  $\text{WTe}_2$ , calculated using the ONCV pseudopotentials, the LDA and the GGA-PBE exchange-correlation functional, and without spin-orbit coupling.

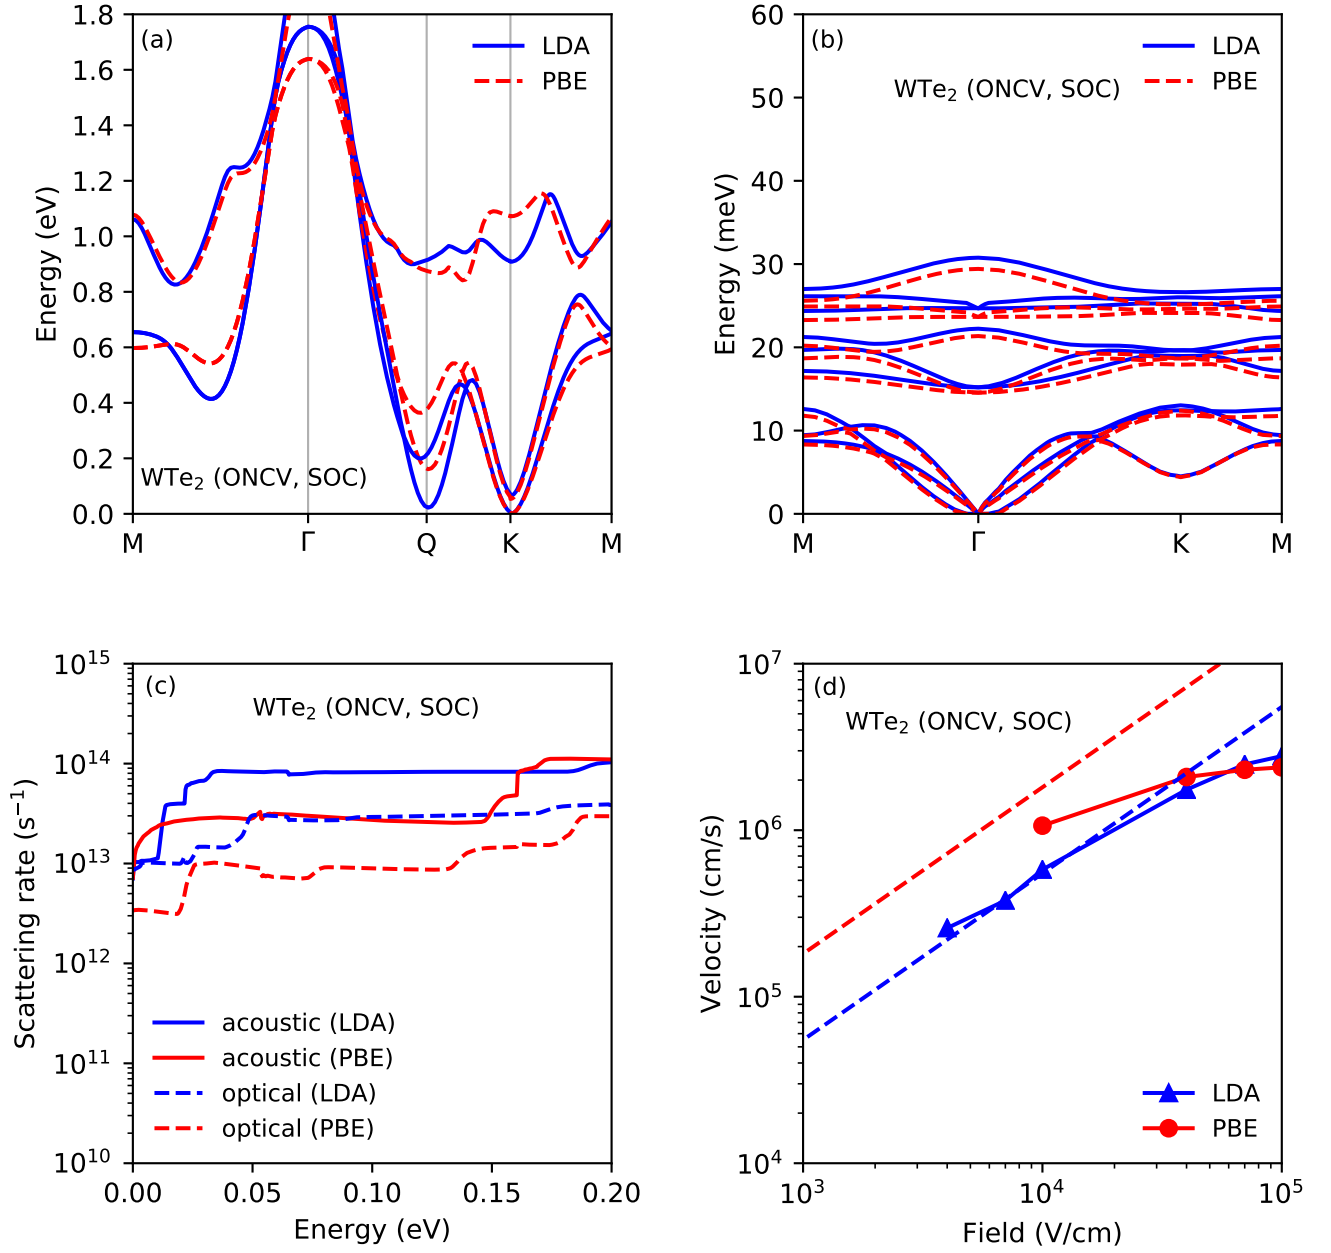

Figure S.20. (a) The electronic bandstructure, (b) phonon dispersion, (c) electron-phonon scattering rates, and (d) velocity-field characteristics for  $\text{WTe}_2$ , calculated using the ONCV pseudopotentials, the LDA and the GGA-PBE exchange-correlation functional, and with spin-orbit coupling.
